# Supplementary material for: Offline Reinforcement Learning: Role of State Aggregation and Trajectory Data
Source: arXiv:2403.17091 source file (2024-03-25)
Supplement: Supplementary file 1 [file lower_bound_appendix.tex]

\section{Proof of \pref{thm:instance_lower_bound}} 

\subsection{Construction of Aggregated MDPs}   
%\ayush{@zeyu, can you clear our redundant definitions please!} 
\par Suppose we are given the latent Markov Decision Process $M = (\calZ, \calA, T, H, \rho)$, and also a distribution $\mu$ over $\calZ\times \calA$. $\Phi$ is an aggregated scheme so that every $\sz\in \calZ$ belongs to exact one of $\phi\in \Phi$, written as $\sz\in \phi$ (also all the latent states in $\phi$ should be at the same layer). We further define the aggregated function $\zeta: \calZ\to \Phi$, where for any $\sz\in\phi$, $\zeta(\sz) \triangleq \phi$.

We are also given a policy $\pieval$ over $M$, which satisfies the following assumption.
\begin{assumption}\label{ass: sec-lower-bound-agg}
    For any $\phi\in\Phi$ and any $\sz, \sz'\in\phi$, we always have $\pieval(\sz) = \pieval(\sz')$. In the following when with no ambiguity, we write $\pieval(\phi) \triangleq \pieval(\sz)$ for some $\sz\in\phi$.
\end{assumption}

Under this assumption, we construct two aggregated MDPs.
\begin{definition}[Aggregated MDP]\label{def:sec-lower-bound-aggMDP}
    Suppose the set $\Phiopt \subset \Phi$ attains the maximum in \pref{def:agg-concentrability}. We define aggregated MDPs $\agg{M}\ind{1} = (\Phi, \calA, \agg{T}, \agg{r}\ind{1}, H, \agg{\rho})$ and $\agg{M}^{(2)} = (\Phi, \calA, \agg{T}, \agg{r}\ind{2}, H, \agg{\rho})$ as follows: transition model $\agg{T}$ is defined as $\agg{T}(\phi\mid\phi, \sa)\triangleq \agg{T}(\phi\mid\phi, \sa; \agg{M})$, where $\agg{T}(\phi\mid\phi, \sa; \agg{M})$ is given in \pref{eq:agg-transition-model}, reward functions are defined as %\ayush{Please change all \(\indic[\cdot]\) to \(\indic\crl{\cdot}\); the latter is a cleaner notation} 
    \begin{align*}
    \agg{r}\ind{1}(\phi, \sa) = \frac{\epsilon}{2H\sum_{\phi\in \Phiopt}\agg{d}^\pieval(\phi)} \cdot \indic\{\phi\in \Phiopt, \sa = \pieval(\phi)\}, \intertext{and,}
    \agg{r}\ind{2}(\phi, \sa) =  - \frac{\epsilon}{2H\sum_{\phi\in \Phiopt}\agg{d}^\pieval(\phi)} \cdot \indic\{\phi\in \Phiopt, \sa = \pieval(\phi)\}.
    \end{align*}
    Initial distribution $\agg{\rho}$ is defined as $\agg{\rho}(\phi)\triangleq \sum_{\sz\in \phi}\rho(\sz)$.
\end{definition}
    We use  $\agg{d}^\pieval(\phi)$ to denote the occupancy measure of \(\phi\) for the policy \(\pieval\) under the dynamics \(\agg{T}\). The value functions and $Q$-functions of $\agg{M}\ind{1}, \agg{M}^{2}$ under the policy $\pieval$ are denoted by $\agg{V}\ind{1}, \agg{V}\ind{2}$ and $\agg{Q}\ind{1}, \agg{Q}\ind{2}$ respectively. Then we have %\ayush{It is not clear from the following three equations whether \( \agg{V}\ind{1}\) is a scalar or a function?} 
\begin{equation}\begin{aligned}\label{eq:sec-lower-bound-value}
    \agg{V}\ind{1}(\agg{\rho}) & = \sum_{\phi\in \Phi} r\ind{1}(\phi, \pieval(\phi))\agg{d}^\pieval(\phi) = \frac{\epsilon}{2H},\\
    \agg{V}\ind{2}(\agg{\rho}) & = \sum_{\phi\in \Phi} r\ind{2}(\phi, \pieval(\phi))\agg{d}^\pieval(\phi) = - \frac{\epsilon}{2H}.\\
\end{aligned}\end{equation}
And for every $\phi\in \Phi$, it is easy to see \CW{Maybe not?}
\begin{equation}\label{eq:sec-lower-bound-bound}
    0\le \agg{V}\ind{1}(\phi)\le \frac{\epsilon}{2H},\qquad  -\frac{\epsilon}{2H}\le \agg{V}\ind{2}(\phi)\le 0.
\end{equation}

\subsection{Construction of Latent-State MDPs} 
Based on $\agg{M}\ind{1}$ and $\agg{M}\ind{2}$, we construct two modified latent-state MDPs $M\ind{1}$ and $M\ind{2}$ as follows:
\begin{align*}
M\ind{1} &= (\calZ', \cA, T\ind{1}, r\ind{1}, H, \rho), \\
M\ind{2} &= (\calZ', \calA, T\ind{2}, r\ind{2}, H, \rho). 
\end{align*}
where \(\cZ' = \cup_{h=1}^H\cZ'_h\) such that the state space \(\cZ'_h = \cZ_h \cup \crl{\su_h, \sv_h, \sw_h}\) contains three extra states \(\crl{\su_h, \sv_h, \sw_h}\) in each layer \(h\). Here $\sw_h$ serves as "terminal state", which can only be transitted from $\su_{h-1}, \sv_{h-1}, \sw_{h-1}$, and under state $\su_{h-1}, \sv_{h-1}, \sw_{h-1}$, taking any action can only transit to $\sw_{h}$ with probability $1$.

\par The reward functions $r\ind{1}, r\ind{2}$ are set to be: 
\begin{align*}
r\ind{1}(\sz, \sa) & = \begin{cases}
    \agg{r}\ind{1}(\zeta(\sz), \sa) & \text{for}~\sz \in \calZ\\ 
    1 & \text{for}~ \sz = \su_h \\  
    - 1 & \text{for}~ \sz = \sv_h \\ 
    0 & \text{for}~ \sz = \sw_h \\ 
\end{cases},
\intertext{and,} \quad r\ind{2}(\sz, \sa) &= \begin{cases}
    \agg{r}\ind{2}(\zeta(\sz), \sa) & \text{for}~\sz \in \calZ \\ 
    1 & \text{for}~ \sz = \su_h \\  
    - 1 & \text{for}~ \sz = \sv_h \\ 
    0 & \text{for}~ \sz = \sw_h \\ 
\end{cases}. 
\end{align*}
Notice that according to this definition, $r\ind{1}(\sz)$ have the same value for all $\sz\in\phi$, and so is $r\ind{2}$. The transition functions $T\ind{1}, T\ind{2}$ for any states $\sz\in \calZ_h, \sz'\in \calZ_{h+1}$ and action $\sa\in\calA$ are set to be
\begin{equation}\label{eq:sec-lower-bound-trans}
    T\ind{1}(\sz'\mid \sz, \sa) = T\ind{2}(\sz'\mid \sz, \sa) = \left(1 - \frac{2}{H}\right) T(\sz'\mid \sz, \sa). 
\end{equation}
Furthermore, we design transitions to $\su_{h+1}, \sv_{h+1}$ so that the value functions of $\sz$ under $M\ind{1}$ (or $M\ind{2}$) matches the value functions of $\zeta(\sz)$ under $\agg{M}\ind{1}$ (or $\agg{M}\ind{2}$). This will imply choices for $i\in\{1, 2\}$,
%\CW{maybe explain a bit the goal of the following before giving intimidating definitions below. E.g., in the original writeup, I first wrote what equations we want to satisfy  according to (a) and (c), and then the solution come up naturally. Probably easier to follow than first giving solutions and verify it. (Just personal taste and no need to follow)}
\begin{equation}\label{eq:sec-lower-bound-transition}\begin{aligned}
    T\ind{i}(\su_{h+1}\mid \sz,\sa) & = \frac{\sum_{\phi'} \agg{T}(\phi'\mid \zeta(\sz), \sa)\agg{V}\ind{i}(\phi') - \sum_{\sz'} T\ind{i}(\sz'\mid \sz,\sa)\agg{V}\ind{i}(\zeta(\sz'))}{2} + \frac{1}{H},\\
    T\ind{i}(\sv_{h+1}\mid \sz,\sa) & = - \frac{\sum_{\phi'} \agg{T}(\phi'\mid \zeta(\sz), \sa)\agg{V}\ind{i}(\phi') - \sum_{\sz'} T\ind{i}(\sz'\mid \sz,\sa)\agg{V}\ind{i}(\zeta(\sz'))}{2} + \frac{1}{H}, \\
\end{aligned}\end{equation}
With these choices of $T\ind{1}$ and $T\ind{2}$, it is easy to see that for $i\in \{1, 2\}$,
\begin{equation}\label{eq:sec-lower-bound-tequal}
    T\ind{i}(\su_{h+1}\mid \sz,\sa) + T\ind{i}(\sv_{h+1}\mid \sz,\sa) = \frac{2}{H}, 
\end{equation}
Furthermore, \pref{eq:sec-lower-bound-bound} gives that $T\ind{i}(\sz'\mid \sz,\sa)$ for all $\sz\in\calZ_{h}, \sa\in\calA, \sz'\in\calZ_{h+1}\cup\{\su_{h+1}, \sv_{h+1}, \sw_{h+1}\}$. \CW{gives what?} Hence both $T\ind{1}$ and $T\ind{2}$ are valid transition models.

\par For MDPs $M\ind{1}$ and  $M\ind{2}$, we have the following properties on value / $Q$-function and occupancies.

\begin{proposition}\label{prop:sec-lower-bound-latent-MDP}
    The following properties hold for $M\ind{1}$ and $M\ind{2}$: 
    \begin{enumerate}[label=\((\alph*)\)]
        \item \label{lem:sec-lower-bound-latent-MDP-a} Suppose the Q-functions of $M\ind{1}$ and $M\ind{2}$ under $\pieval$ are $Q\ind{1}$ and $Q\ind{2}$, then for any $\phi\in \Phi$ and $\sz\in \phi, a\in \calA$, we have
        $$Q\ind{1}(\sz, \sa) = \agg{Q}\ind{1}(\zeta(\sz), \sa), \quad Q\ind{2}(\sz, \sa) = \agg{Q}\ind{2}(\zeta(\sz), \sa).$$
        \item \label{lem:sec-lower-bound-latent-MDP-b} Suppose the value functions of $M\ind{1}, M\ind{2}$ under policy $\pieval$ to be $V\ind{1}, V\ind{2}$, then we have
        $$V\ind{1}(\rho) - V\ind{2}(\rho) = \frac{\epsilon}{H}.$$ 
        \item \label{lem:sec-lower-bound-latent-MDP-c} For any $\phi\in \Phi$, action $\sa\in\calA$ and latent state $\sz'\in\calZ'$, we have
        $$\sum_{\sz\in \phi}\mu(\sz\mid \sz\in \phi, \sa)T\ind{1}(\sz'\mid \sz, \sa) = \sum_{\sz\in \phi}\mu(\sz\mid \sz\in \phi, \sa)T\ind{2}(\sz'\mid \sz, \sa).$$
        \item \label{lem:sec-lower-bound-latent-MDP-d} For any $\sz\in\calZ$, suppose the occupancies of policy $\pi$ under $M, M\ind{1}$ and $M\ind{2}$ are $d^\pi(\cdot; M)$, $d^\pi(\cdot; M\ind{1})$ and $d^\pi(\cdot; M\ind{2})$. Then we have for any $\sz\in\calZ$ and $i\in\{1, 2\}$,
        $$\frac{1}{16}d^\pi(\sz; M)\le d^\pi(\sz; M\ind{i})\le d^\pi(\sz; M).$$
    \end{enumerate}
\end{proposition}
\begin{proof}[ {Proof of \pref{prop:sec-lower-bound-latent-MDP}}]
We verify each part separately below. We first observe that for any $h$ and $\sa\in\calA$, we have
\begin{align*}
    Q\ind{1}(\su_h, \sa) &= Q\ind{2}(\su_h, \sa) = 1,\\
    Q\ind{1}(\sv_h, \sa) &= Q\ind{2}(\sv_h, \sa) = -1,\\
    Q\ind{1}(\sw_h, \sa) &= Q\ind{2}(\sw_h, \sa) = 0.
\end{align*} 

\paragraph{Proof of \ref{lem:sec-lower-bound-latent-MDP-a}: } We use induction from the last layer to the first. Without loss of generality we only verify the first equation, and the proof of the second equation is similar. For $(\sz, \sa)$ in layer $H$, we have $Q_1^\pieval(\sz, \sa) = 0 = \agg{Q}_1^\pieval(\zeta(\sz), \sa)$. Next, suppose for layer $h+1$, \ref{lem:sec-lower-bound-latent-MDP-a} holds. Then for layer $h$, according to Bellman equation, we have
\begin{align*}
    Q_1^{\pieval}(\sz, \sa) & = r\ind{1}(\sz, \sa) + T\ind{1}(\su_{h+1}\mid \sz,\sa) - T\ind{1}(\sv_{h+1}\mid \sz,\sa) + \sum_{\sz'} T\ind{1}(\sz'\mid \sz,\sa)Q_1^\pieval(\sz', \pieval(\sz'))\\
    & = \agg{r}_1(\zeta(\sz), \sa) + T\ind{1}(\su_{h+1}\mid \sz,\sa) - T\ind{1}(\sv_{h+1}\mid \sz,\sa) + \sum_{\sz'} T\ind{1}(\sz'\mid \sz,\sa)\agg{V}\ind{1}(\zeta(\sz'))\\
    & = \agg{r}_1(\zeta(\sz), \sa) + \sum_{\phi'} \agg{T}(\phi'\mid \zeta(\sz), \sa)\agg{V}\ind{1}(\phi') = \agg{Q}_1^\pieval(\zeta(\sz), \sa),
\end{align*}
%\ayush{here as well make the conclusion clear by separating it into a new line}
In the last equation we use Bellman equation under $\agg{M}\ind{1}$. This completes the induction at layer $h$. Therefore, we have $Q_1^{\pieval}(\sz, \sa) = \agg{Q}_1^\pieval(\zeta(\sz), \sa)$ for all $\sz\in \calZ$ and \ref{lem:sec-lower-bound-latent-MDP-a} is verified.

\paragraph{Proof of \ref{lem:sec-lower-bound-latent-MDP-b}: } According to \ref{lem:sec-lower-bound-latent-MDP-a}, and also \pref{ass: sec-lower-bound-agg}, we have
\begin{align*} 
    V\ind{1}(\sz) = Q\ind{1}(\sz, \pieval(\sz)) = \agg{Q}\ind{1}(\zeta(\sz), \pieval(\zeta(\sz))) = \agg{V}\ind{1}(\zeta(\sz)).
\end{align*}
Similarly, we also get $V\ind{2}(\sz) = \agg{V}\ind{2}(\zeta(\sz))$. We further notice from \pref{eq:sec-lower-bound-value}, we have
$$\agg{V}\ind{1}(\agg{\rho}) - \agg{V}\ind{2}(\agg{\rho}) = \frac{\epsilon}{H}.$$
This implies
$$V\ind{1}(\rho) - V\ind{2}(\rho) = \frac{\epsilon}{H}.$$

\paragraph{Proof of \ref{lem:sec-lower-bound-latent-MDP-c}: } For those $\sz'\not\in \{\su_h, \sv_h\}_{h=1}^H$, we always have $T\ind{1}(\sz'\mid \sz, \sa) = T\ind{2}(\sz'\mid\sz, \sa)$ according to \pref{eq:sec-lower-bound-transition}, and hence the equation holds. As for $\sz' = \su_h$, according to \pref{eq:sec-lower-bound-tequal}, we only need to verify $\sum_{\sz\in \phi} \mu(\sz, \sa)(T\ind{1}(\su_h\mid\sz, \sa) - T\ind{2}(\su_h\mid\sz, \sa)) = 0$. Actually we have
%\ayush{Poor Indentation in the first line. See how I fixed it in the following text. Please do the same at other places.} 
\begin{align*}
    \hspace{0.5in}&\hspace{-0.5in}\quad \sum_{\sz\in \phi} \mu(\sz, \sa)(T\ind{1}(\su_h\mid\sz, \sa) - T\ind{2}(\su_h\mid\sz, \sa))\\
    & = \sum_{\sz\in \phi} \mu(\sz, \sa)\big(\sum_{\phi'} \agg{T}(\phi'\mid \zeta(\sz), \sa)\agg{V}\ind{1}(\phi') - \sum_{\sz'} T\ind{1}(\sz'\mid \sz,\sa)\agg{V}\ind{1}(\zeta(\sz'))\big)\\
    & = \sum_{\sz\in \phi} \mu(\sz, \sa)\sum_{\phi'} \agg{T}(\phi'\mid \phi, \sa)\agg{V}\ind{1}(\phi') - \sum_{\phi'}\sum_{\sz'\in \phi'} \agg{V}\ind{1}(\zeta(\sz'))\sum_{\sz\in \phi} \mu(\sz, \sa)T\ind{1}(\sz'\mid \sz,\sa)\\
    & = \sum_{\sz\in \phi} \mu(\sz, \sa)\sum_{\phi'} \agg{T}(\phi'\mid \phi, \sa)\agg{V}\ind{1}(\phi') - \sum_{\phi'}\agg{V}\ind{1}(\phi')\sum_{\sz'\in \phi'} \sum_{\sz\in \phi} \mu(\sz, \sa)T\ind{1}(\sz'\mid \sz,\sa)\\
    & = \sum_{\sz\in \phi} \mu(\sz, \sa)\sum_{\phi'} \agg{T}(\phi'\mid \phi, \sa)\agg{V}\ind{1}(\phi') - \sum_{\phi'}\agg{V}\ind{1}(\phi')\sum_{\sz\in \phi} \mu(\sz, \sa)\agg{T}(\phi'\mid \phi, \sa) = 0.
\end{align*}
%\ayush{General tip: whenever the math block looks so big and ugly always separate the conclusion in a new line so that it is clear; see what I did above.} 
In the second last equation we use the definition of $\agg{T}$ in \pref{eq:agg-transition-model}. Hence \ref{lem:sec-lower-bound-latent-MDP-c} is verified for $\sz' = \su_h$. The proof for $\sz' = \sv_h$ is similar.

\paragraph{Proof of \ref{lem:sec-lower-bound-latent-MDP-d}: } Without loss of generality we only verify the result for $M\ind{1}$. We will prove via induction on $h$ that for any $\sz\in\calZ_{h}$, we have
$$\left(\frac{H-2}{H}\right)^{h-1} d^\pi(\sz; M)\le d^\pi(\sz, M\ind{1})\le d^\pi(\sz, M).$$
For $h = 1$, we have $d^\pi(\sz; M) = \rho(\sz) = d^\pi(\sz; M\ind{1})$ for any $\sz\in\calZ_1$. Next we go from $h$ to $h+1$. For any $\sz\in\calZ_{h+1}$, we write
\begin{align*}
    d^\pi(\sz; M\ind{1}) = \sum_{\sz'\in\calZ_h}d^\pi(\sz'; M\ind{1})T\ind{1}(\sz\mid\sz', \pi(\sz')).
\end{align*}
Additionally, \pref{eq:sec-lower-bound-trans} gives that
$$T\ind{1}(\sz\mid\sz', \pi(\sz')) = \frac{H-2}{H}T(\sz\mid\sz', \pi(\sz')).$$
This together with induction hypothesis implies
\begin{align*}
    d^\pi(\sz; M\ind{1}) & \le \sum_{\sz'\in\calZ_h}d^\pi(\sz'; M)T(\sz\mid\sz', \pi(\sz')) = d^\pi(\sz, M),\\
    d^\pi(\sz; M\ind{1}) & \ge \left(\frac{H-2}{H}\right)^{h-1}\sum_{\sz'\in\calZ_h}d^\pi(\sz'; M)\cdot \frac{H-2}{H}T(\sz\mid\sz', \pi(\sz')) = \left(\frac{H-2}{H}\right)^{h}d^\pi(\sz, M),
\end{align*}
which proves the induction hypothesis of $h+1$.
\end{proof}

\subsection{Construction of Rich-Observation MDPs} 
\par Our next job is to lift latent state MDPs $M\ind{1}$ and $M\ind{2}$ into rich observations.
\par We first construct the rich observation state space $\calX = \bigcup_{h=1}^H\calX_h$, which is also separated into disjoint sets $\calX(\phi)$ for each $\phi\in \Phi$, with
\begin{equation}
|\calX(\phi)|\ge  \frac{32|\phi|^4H^3\ophatC{M}{\mu}{\epsilon}{\Phi}^3}{\epsilon^3}.	 \label{eq:rich_count} 
\end{equation}

%\ayush{I think you should  model the decoder function  by \(\psi\) instead of modeling the emission function.} 
Every decoder function $\psi$ is a mapping from $\calX$ into $\calZ$. We define the set of decoder functions $\Psi$ as follows:
\begin{align}\label{eq:sec-lower-bound-defPsi}
    \Psi\triangleq \{\psi\mid \forall \phi, \psi^{-1}(\sz): \sz\in \phi \text{ is a partition of } \calX(\phi) \text{ with }|\psi^{-1}(\sz)| = \nicefrac{|\calX|}{|\phi|}\}.
\end{align}
This set $\Psi$ includes all possible decoder function where for all latent states within each aggregated state, the size of rich observations mapping to these latent states should be the same.
%\CW{This definition is hard to understand. Should explain more in words. }
For every $\psi\in \Psi$ we use $\calX_\psi(\sz)$ to denote $\psi^{-1}(\sz)$. Then we have for any $\sz\in \phi$, $|\calX_\psi(\sz)| = \nicefrac{|\calX(\phi)|}{|\phi|}$. To facilitate the proof, we further define $\psi(\su_h) = \su_h, \psi(\sv_h) = \sv_h$ and $\psi(\sw_h) = \sw_h$ and $\calX_\psi(\su_h) = \{\su_h\}, \calX_\psi(\sv_h) = \{\sv_h\}$ and $\calX_\psi(\sw_h) = \{\sw_h\}$ for all $\psi\in \Psi$. 

%\ascomment{For the ease of notation, we overload and define \(\calX_\psi(\sx) = \calX_\psi(\sz)\) where \(\sz = \psi(\sx)\).} 

\par Next, for every $\psi\in \Psi$, we construct rich observation MDP $\rich{M}_{\psi}\ind{1} = (\calX, \calA, \rich{T}_\psi\ind{1}, \rich{R}_\psi\ind{1}, H, \rich{\rho})$ and $\rich{M}_{\psi}\ind{1} = (\calX, \calA, \rich{T}_\psi\ind{1}, \rich{R}_\psi\ind{1}, H, \rich{\rho})$ based on $M\ind{1}, M\ind{2}$ and the decoder function $\psi$: the state space is defined as $\calX = \cup_{\phi\in \Phi} \calX(\phi)\cup\{\su_h, \sv_h, \sw_h\}_{h=1}^H$. For any $\sx\in \calX_\psi(\sz)$ and $\sx'\in \calX_\psi(\sz')$, we define transition%\ayush{The following is ugly. Clean it!} 
\begin{equation}\label{eq:sec-lower-bound-def-T}
    \rich{T}_\psi\ind{1}(\sx'\mid\sx, \sa) \triangleq \frac{T\ind{1}(\sz'\mid \sz, \sa)}{|\calX_\psi(\sz')|} \quad\text{and}\quad \rich{T}_\psi^2(\sx'\mid\sx, \sa) \triangleq \frac{T\ind{2}(\sz'\mid \sz, \sa)}{|\calX_\psi(\sz')|},
\end{equation}
and rewards $\rich{R}\ind{1}(\cdot\mid\sx, \sa), \rich{R}\ind{2}(\cdot\mid\sx, \sa)\in\Delta(\{-1, 1\})$ with expectation to be 
\begin{equation}\label{eq:sec-lower-bound-def-r}
    r\ind{1}(\sz, \sa) \quad\text{and}\quad  r\ind{2}(\sz, \sa),
\end{equation}
and initial distribution
\begin{equation}\label{eq:sec-lower-bound-def-rho}
    \rich{\rho}(\sx)\triangleq \frac{\rho(\sz)}{|\calX_\psi(\sz)|}.
\end{equation}
The data collection distribution defined as
\begin{equation}\label{eq:sec-lower-bound-defmu}
    \rich{\mu}_\psi(\sx, \sa) = \frac{\mu(\sz, \sa)}{|\calX_\psi(\sz)|},
\end{equation}
and we use $\mu_{\psi, h}$ to denote the marginal distribution conditioned on $\sx\in \calX_h$. The policy $\ripieval$ to be evaluated is defined as
$$\ripieval(\sx) = \pieval(\sz).$$ 

We have the following propositions about $Q$-functions and occupancy measures of $\rich{M}_\psi\ind{1}$ and $\rich{M}_\psi\ind{2}$.
\begin{proposition}\label{prop:sec-lower-bound-Q}
    Suppose the $\rich{Q}_\psi\ind{1}$ and $\rich{Q}_\psi\ind{2}$ are $Q$-functions, and $\rich{V}_\psi\ind{1}$ and $\rich{V}_\psi\ind{2}$ are value functions of $\rich{M}_\psi\ind{1}$ and $\rich{M}_\psi\ind{2}$ under policy $\ripieval$. Then we have 
    \begin{enumerate}[label=\((\alph*)\)]
        \item \label{lem:sec-lower-bound-Q-1} $\rich{Q}_\psi\ind{1}$ and $\rich{Q}_\psi\ind{2}$, $\rich{V}_\psi\ind{1}$ and $\rich{V}_\psi\ind{2}$ are independent of $\psi$. In the following text, when without ambiguity, we denote the two $Q$-functions as $\rich{Q}\ind{1}$ and $\rich{Q}\ind{2}$, and the two value functions as $\rich{V}\ind{1}$ and $\rich{V}\ind{2}$.
        \item \label{lem:sec-lower-bound-Q-2} For any $1\le h\le H$, we have 
        $$\sum_{\sx}\rich{\mu}_{\psi, h}(\sx, \ripieval(\sx))\rich{Q}_\psi\ind{1}(\sx, \ripieval(\sx))\quad \text{and}\quad \sum_{\sx}\rich{\mu}_{\psi, h}(\sx, \ripieval(\sx))\rich{Q}_\psi\ind{2}(\sx, \ripieval(\sx))$$
        is independent of $\psi$. In the following text, when without ambiguity, we denote these two values as $(\mu Q)_h\ind{1}$ and $(\mu Q)_h\ind{2}$.
        \item \label{lem:sec-lower-bound-Q-3} For any policy $\pi$ on MDP $M\ind{1}$ (or $M\ind{2}$), let policy $\rich{\pi}$ on $\rich{M}_\psi\ind{1}$ (or $\rich{M}_\psi\ind{2}$) is defined as $\rich{\pi}(\sx) = \pi(\psi(\sx))$ for any $\sx\in\calX$. Suppose the occupancy measure of policy $\pi$ under $M\ind{1}$ and $M\ind{2}$ to be $d\ind{1}(\cdot)$ and $d\ind{2}(\cdot)$, and the occupancy measure of policy $\rich{\pi}$ under $\rich{M}_\psi\ind{1}$ and $\rich{M}_\psi\ind{2}$ to be $\rich{d}_\psi\ind{1}(\cdot)$ and $\rich{d}_\psi\ind{2}(\cdot)$. Then we have for any $\sx\in\calX_\psi(\sz)$,
        \begin{equation}\label{eq:sec-lower-bound-Q-3}
            \rich{d}_\psi\ind{1}(\sx) = \frac{d\ind{1}(\sz)}{|\calX_\psi(\sz)|}\quad \text{and}\quad \rich{d}_\psi\ind{2}(\sx) = \frac{d\ind{2}(\sz)}{|\calX_\psi(\sz)|}.
        \end{equation}
    \end{enumerate}
\end{proposition}
\begin{proof}[Proof of Proposition \ref{prop:sec-lower-bound-Q}] 
    Without loss of generality, in the following we only prove the results for $\rich{Q}_\psi\ind{1}$, and the proofs of results for $\rich{Q}_\psi\ind{2}$ is are similar.

    \paragraph{Proof of \ref{lem:sec-lower-bound-Q-1}: } We only need to verify that for any $\psi\in\Psi$, $\phi\in \Phi$ and $\sx\in\calX(\phi)$, we always have 
    \begin{equation}\label{eq:sec-lower-bound-eqQ}
        \rich{Q}_\psi\ind{1}(\sx, \sa) = \agg{Q}\ind{1}(\phi, \sa).
    \end{equation} Suppose $\phi\in\Phi_h$, we prove this results by induction from $h = H$ to $h = 1$. When $h = H$, we have $\rich{Q}_\psi\ind{1}(\sx, \sa) = \agg{Q}\ind{1}(\phi, \sa) = 0$, and \pref{eq:sec-lower-bound-eqQ} holds. Next, suppose \pref{eq:sec-lower-bound-eqQ} holds for $h+1$, then $\phi\in\Phi_h$ and any $\sx\in \calX(\phi)$, according to Bellman equation we have
    \begin{align*}
        \rich{Q}_\psi\ind{1}(\sx, \sa) = \rich{r}_\psi\ind{1}(\sx, \sa) + \sum_{\sx'\in \calX_{h+1}}\rich{T}_\psi\ind{1}(\sx'\mid\sx, \sa) \rich{Q}_\psi\ind{1}(\sx', \ripieval(\sx')).
    \end{align*}
    Next, we notice that for any $\phi'\in\Phi_{h+1}$ and $\sx'\in\calX(\phi')$, we have $\ripieval(\sx') = \aggpieval(\phi')$, hence according to \pref{eq:sec-lower-bound-def-T}, \pref{eq:sec-lower-bound-def-r} and the induction hypothesis, we have
    \begin{align*}
        \rich{Q}_\psi\ind{1}(\sx, \sa) & = r\ind{1}(\psi(\sx), \sa) + \sum_{\phi\in\Phi_{h+1}}\agg{Q}\ind{1}(\phi, \aggpieval(\phi))\sum_{\sx'\in \calX_{h+1}(\phi')}\rich{T}_\psi\ind{1}(\sx'\mid\sx, \sa)\\
        & = r\ind{1}(\psi(\sx), \sa) + \sum_{\phi\in\Phi_{h+1}}\agg{Q}\ind{1}(\phi, \aggpieval(\phi))\sum_{\sz'\in \phi'}T\ind{1}(\sz'\mid\psi(\sx), \sa).
    \end{align*}
    Finally, noticing that for any $\sz'\in\phi'$ we always have $\pieval(\sz') = \aggpieval(\phi')$, according to \ref{lem:sec-lower-bound-latent-MDP-a} in \pref{prop:sec-lower-bound-latent-MDP}, we have, $Q\ind{1}(\sz', \pieval(\sz')) = \agg{Q}\ind{1}(\phi', \aggpieval(\phi'))$. Therefore, using Bellman equation for $M\ind{1}$, we obtain
    \begin{align*}
        \rich{Q}_\psi\ind{1}(\sx, \sa) & = r\ind{1}(\psi(\sx), \sa) + \sum_{\phi\in\Phi_{h+1}}\sum_{\sz'\in \phi'}T\ind{1}(\sz'\mid\psi(\sx), \sa)Q\ind{1}(\sz', \pieval(\sz'))\\
        & = r\ind{1}(\psi(\sx), \sa) + \sum_{\sz'\in \calZ_{h+1}}T\ind{1}(\sz'\mid\psi(\sx), \sa)Q\ind{1}(\sz', \pieval(\sz'))\\
        & =  Q\ind{1}(\psi(\sx), \sa) = \agg{Q}\ind{1}(\phi, \sa),
    \end{align*}
    where in the last equation we again use \ref{lem:sec-lower-bound-latent-MDP-a} in \pref{prop:sec-lower-bound-latent-MDP}. This finishes the proof of induction hypothesis for $h$.

    \paragraph{Proof of \ref{lem:sec-lower-bound-Q-2}: } We first notice that fix $\phi\in \Phi_h$, for any $\sx\in\calX(\phi)$, we have $\ripieval(\sx) = \pieval(\sz) = \aggpieval(\phi)$. Hence according to \ref{lem:sec-lower-bound-Q-1}, for any $\sx\in\calX(\phi)$, we have $\rich{Q}_\psi\ind{1}(\sx, \ripieval(\sx)) = \agg{Q}\ind{1}(\phi, \aggpieval(\phi))$. Therefore, we only need to verify that 
    $$\sum_{\sx\in\calX(\phi)}\rich{\mu}_{\psi, h}(\sx, \ripieval(\sx)) = \sum_{\sx\in\calX(\phi)}\rich{\mu}_{\psi, h}(\sx, \aggpieval(\phi))$$
    is independent of $\psi$. Actually, \pref{eq:sec-lower-bound-defmu} gives that
    \begin{align*}
        \sum_{\sx\in\calX(\phi)}\rich{\mu}_{\psi, h}(\sx, \aggpieval(\phi)) & = \sum_{\sz\in\phi}\sum_{\sx\in\calX_{\psi}(\sz)}\rich{\mu}_{\psi, h}(\sx, \aggpieval(\phi)) = H\cdot \sum_{\sz\in\phi}\sum_{\sx\in\calX_{\psi}(\sz)}\rich{\mu}_{\psi}(\sx, \aggpieval(\phi))\\
        & = H\cdot \sum_{\sz\in\phi} \mu(\sz, \aggpieval(\phi)),
    \end{align*}
    which is independent of $\psi$.

    \paragraph{Proof of \ref{lem:sec-lower-bound-Q-3}: } We will prove via induction on the layer of $\sx$. For $\sx\in\calX_1$, \pref{eq:sec-lower-bound-Q-3} holds acording to initial distribution definition \pref{eq:sec-lower-bound-def-rho}. Additionally, the induction from layer $h$ to layer $h+1$ can be achieved by
    $$\rich{d}_\psi\ind{1}(\sx) = \sum_{\sx'\in\calX_h} \rich{d}_\psi\ind{1}(\sx')\rich{T}(\sx\mid\sx', \rich{\pi}(\sx')) =\sum_{\sz'\in\calZ_h} d\ind{1}(\sz')\frac{T(\sz\mid\sz', \pi(\sz'))}{|\calX_\psi(\sz)|} = \frac{d\ind{1}(\sz)}{|\calX_\psi(\sz)|}$$
    for any $\sx\in\sz$ and $\sz\in\calZ_{h+1}$.
\end{proof}

\subsection{Proof of \pref{thm:instance_lower_bound}} 
\par We further use $\mathbb{P}_n^{\rich{M}_\psi\ind{1}}, \mathbb{P}_n^{\rich{M}_\psi\ind{2}}$ to denote the distribution of the $n$-sample offline dataset, if the underlying MDP is $\rich{M}_\psi\ind{1}$ or $\rich{M}_\psi\ind{2}$. And we define
$$\mathbb{P}_n\ind{1} = \frac{1}{|\Psi|}\sum_{\psi\in \Psi} \mathbb{P}_n^{\rich{M}_\psi\ind{1}} \quad\text{and}\quad \mathbb{P}_n\ind{2} = \frac{1}{|\Psi|}\sum_{\psi\in \Psi} \mathbb{P}_n^{\rich{M}_\psi\ind{2}}.$$

For any $\rich{M} = \rich{M}_\psi\ind{1}$ or $\rich{M}_\psi\ind{2}$, we use $D_n\sim \rich{M}$ to denote the size-$n$ dataset where each element $(\sx, \sa, r, \sx')$ are i.i.d.~ samples according to the following process: first sample $(\sz, \sa)\sim \rich{\mu}_\psi$, then collect $r\sim \rich{R}\ind{1}(\cdot\mid\sx, \sa), \sx'\sim \rich{T}_\psi\ind{1}(\sx'\mid \sx, \sa)$ (or $r\sim \rich{R}\ind{1}(\cdot\mid\sx, \sa), \sx'\sim \rich{T}_\psi^2(\sx'\mid \sx, \sa)$).

\begin{definition}[$W$-function]
    For a given MDP $M = (\calX, \calA, T, r, H, \rho)$ where $\calX = \bigcup_{h=1}^H \calX_h$, a distribution $\mu$ of state space and policy $\pieval$, we define the $W$-function: $[H]\to \mathbb{R}$ with respect to $\mu, M$ as
    $$W(h; \mu, M) = \sum_{\sx\in\calX_h}\mu_h(\sx)V^\pieval(\sx; M),$$
    where $\mu_h$ is the marginal distributon of $\mu$ over $\calX_h$, and $V^\pieval(\cdot; M)$ is the value function of $M$ under policy $\pieval$.
\end{definition}

Then we have the following theorem:

\begin{theorem}\label{thm:sec-lower-bound}
    Given any MDP $M$, aggregation scheme $\Phi$, offline distribution $\mu$, evaluation policy \(\pieval\), there exists a family  
    \begin{align*}
    \cG = \prn*{\rich{M},\ripieval, \rich{\mu}(\cdot; \rich{M}), \rich{\cF}}, 
    \end{align*}
    of offline policy evaluation problems where
    \begin{enumerate}[label=\(\bullet\)]
        \item $\check{M}$ is an MDP with rich observations whose latent state dynamics are based on \(M\), 
        \item \(\check \pieval\) is an evaluation policy and is the same for all instances in \(\cG\), 
        \item \(\rich{\mu}(\cdot; \rich{M})\) is an offline distribution that satisfies $\tabC_\epsilon(\ripieval, \rich \mu(\cdot; \rich M); \rich M) \leq 2 \tabC_\epsilon( \pieval, \mu; M)$,  
        \item $\abs{\rich{\cF}} \leq 2$ and is same for all instances in \(\cG\). Furthermore, for each \(\check M\), the class \(\rich{\cF}\) realizes the tuple \((Q^{\ripieval}(\cdot; \rich M), \rich{W}(\cdot; \rich \mu,  \rich M))\)  where \(\rich{W}(\sx, \sa; \rich \mu, \rich M)) \ldef{} \rich{\mu}(\sx, \sa; \rich{M}) Q^{\ripieval}(\sx, \sa; \rich M)\),  \ayush{Define this as \(W\) and make a remark somewhere that we are only giving it more information} \ayush{Main body present without \(W\) but prove with \(W\) and restate there!} 
    \end{enumerate}
    such that any offline policy evaluation algorithm that returns the value of \(\check \pieval\) up to \(\epsilon/16H\)-precision needs an offline dataset of size at least 
        \begin{align*} 
N = \Omega\prn*{\frac{H}{\epsilon} \ophatC{M}{\Phi}{\mu}{\epsilon}}. 
\end{align*}
on some problem instance in \(\cG\). %(where the offline dataset is sampled from \(\check \mu(\cdot; \check M)\)). 

% in order 
%     such that any \((N, \nicefrac{\epsilon}{16H})\)-OPE algorithm must fail to evaluate the value of \(\check \pieval\) on some instance \(g \in \cG\) if 
%     \begin{align*}
% N \le \frac{H}{8\epsilon} \ophatC{M}{\Phi}{\mu}{\epsilon}. 
% \end{align*}
 
    % and returns a value $\widehat{V}$, there must exist some $\rich{M}\in\mathcal{M}$ such that %\ayush{Always have brackets with expectation functions!} 
    % $$\mathbb{E}_{D_n\sim \rich{M}}\left[\left|\widehat{V} - V(\rich{M})\right|\right]\ge \frac{\epsilon}{8H},$$
\end{theorem}

\begin{theorem}\label{thm:sec-lower-bound}
    There exists a class $\mathcal{M}$ of lifting MDPs. For any algorithm that takes the following as input:
    \begin{enumerate}
        \item Dataset $D_n$ with $n\le \frac{H}{8\epsilon} \ophatC{M}{\Phi}{\mu}{\epsilon}$;
        \item A class $\mathcal{F}$ of tuples $\mathcal{F} = \{(Q(M), \mu Q(M)): M\in\mathcal{M}\}.$
    \end{enumerate}
    and returns a value $\widehat{V}$, there must exist some $M\in\mathcal{M}$ such that %\ayush{Always have brackets with expectation functions!} 
    $$\mathbb{E}_{D_n\sim M}\left[\left|\widehat{V} - V(M)\right|\right]\ge \frac{\epsilon}{8H},$$
\end{theorem}

\begin{theorem}\label{thm:sec-lower-bound}
     For any algorithm that takes the following as input:
    \begin{enumerate}
        \item Dataset $D_n$ with $n\le \frac{H}{8\epsilon} \ophatC{M}{\Phi}{\mu}{\epsilon}$;
        \item A class $\mathcal{F}$ of tuples
        $$\mathcal{F} = \{(\rich{Q}\ind{1}, (\mu Q)\ind{1}), (\rich{Q}\ind{2}, (\mu Q)^2)\}.$$
    \end{enumerate}
    and returns a value $\widehat{V}_{D_n}$, there must exist some $\check{M}\in \{\rich{M}_\psi\ind{1}: \psi\in \Psi\}\cup\{\rich{M}_\psi\ind{2}: \psi\in \Psi\}$ such that %\ayush{Always have brackets with expectation functions!} 
    $$\mathbb{E}_{D_n\sim \rich{M}}\left[\left|\widehat{V}_{D_n} - \rich V^{\rich{M}}(\rich{\rho})\right|\right]\ge \frac{\epsilon}{8H},$$
    where $\rich V^{\rich{M}}$ denotes the value function of $\rich{M}$.
\end{theorem}
\begin{remark}
    During the data collection process, our current method collects from distribution $\rich{\mu}_\psi$. To incorportate new states $\{\su_h, \sv_h, \sw_h\}_{h=1}^H$, we can change the data collection distribution into $\rich{\mu}_\psi'$ where $\rich{\mu}_\psi'(\sx) = \frac{H-2}{H}\rich{\mu}_\psi(\sx)$ and other portion are properly allocated to $\su_h, \sv_h, \sw_h$. With this new $\rich{\mu}_\psi'$, we can show that the new $\ophatC{\rich{M}_\psi\ind{1}}{\Phi}{\rich{\mu}_\psi'}{\epsilon} = \mathcal{O}(\ophatC{M}{\Phi}{\mu}{\epsilon})$, and also any algorithm requires $\Omega(\ophatC{\rich{M}_\psi\ind{1}}{\Phi}{\rich{\mu}_\psi'}{\epsilon} / \epsilon)$ number of samples to achieve $\epsilon$-close estimation of value functions.
\end{remark}

\par To prove this theorem, we first show the following lemma.
\begin{lemma}
    For any algorithm which takes $D_n = \{(\sx_i,\sa_i, r_i, \sx_i')\}_{i=1}^n$ as input and returns a value $\widehat{V}_{D_n}$, it must satisfy
    $$\sup_{\rich{M}\in \{\rich{M}_\psi\ind{1}: \psi\in \Psi\}\cup\{\rich{M}_\psi\ind{2}: \psi\in \Psi\}}\mathbb{E}_{D_n\sim \rich{M}}\left[\left|\widehat{V}_{D_n} - \rich{V}^{\rich{M}}(\rich{\rho})\right|\right]\ge \frac{\epsilon}{4H}\cdot \left(1 - D_{\mathrm{TV}}(\mathbb{P}_n\ind{1}, \mathbb{P}_n\ind{2})\right).$$
\end{lemma}
\begin{proof}
    For any dataset $D_n$, we use $\delta\prn{D_n}$ to denote the following random variable:
    $$\delta\prn{D_n} = \indic\left\{\widehat{V}_{D_n}\le \frac{\rich{V}\ind{1}(\rich\rho) + \rich{V}\ind{2}(\rich\rho)}{2}\right\},$$
    where $\rich{V}\ind{1}$ and $\rich{V}\ind{2}$ are defined in \ref{lem:sec-lower-bound-Q-1}. Then for $\rich{M}\in \{\rich{M}_\psi\ind{1}: \psi\in \Psi\}$, we have %\ayush{The third line in the following seems wrong / notationally inconsistent!} 
    \begin{align*}
        \mathbb{E}_{D_n\sim \rich{M}}\left|\widehat{V}_{D_n} - \rich{V}^{\rich{M}}(\rich\rho)\right| &\ge \mathbb{E}_{D_n\sim \rich{M}} \left[\delta\prn{D_n}\cdot \left|\widehat{V}_{D_n} - \rich{V}^{\rich{M}}(\rich\rho)\right|\right]\\
        &\ge \mathbb{E}_{D_n\sim \rich{M}}\left[\delta\prn{D_n}\cdot \left|\frac{\rich{V}\ind{1}(\rich\rho) + \rich{V}\ind{2}(\rich\rho)}{2} - \rich{V}\ind{1}(\rich\rho)\right|\right]\\
        & \ge \mathbb{P}_{D_n\sim \rich{M}}(\delta\prn{D_n} = 1)\cdot \frac{\rich{V}\ind{1}(\rich\rho) - \rich{V}\ind{2}(\rich\rho)}{2}\\
        & = \frac{\epsilon}{2H}\cdot \mathbb{P}_{D_n\sim \rich{M}}(\delta\prn{D_n} = 1),
    \end{align*}
    where in the last equation we use \ref{lem:sec-lower-bound-latent-MDP-b} and \ref{lem:sec-lower-bound-Q-1}. Similarly, for $\rich{M}\in \{\rich{M}_\psi\ind{2}: \psi\in \Psi\}$, we have
    $$\mathbb{E}_{D_n\sim \rich{M}}\left[\left|\widehat{V}_{D_n} - \rich{V}^{\rich{M}}(\rich\rho)\right|\right]\ge \mathbb{P}_{D_n\sim \rich{M}}(\delta\prn{D_n} = 0).$$
    Therefore, we obtain that %\ayush{First line indentation in the following} 
    \begin{align*}
        \hspace{0.5in}&\hspace{-0.5in}\quad \sup_{\rich{M}\in \{\rich{M}_\psi\ind{1}: \psi\in \Psi\}\cup\{\rich{M}_\psi\ind{2}: \psi\in \Psi\}}\mathbb{E}_{D_n\sim \rich{M}}\left[\left|\widehat{V}_{D_n} - \rich{V}^{\rich{M}}(\rich\rho)\right|\right]\\
        & \ge \frac{1}{2|\Psi|}\sum_{\rich{M}\in \{\rich{M}_\psi\ind{1}: \psi\in \Psi\}}\mathbb{E}_{D_n\sim \rich{M}}\left[\left|\widehat{V}_{D_n} -\rich{V}^{\rich{M}}(\rich\rho)\right|\right] + \frac{1}{2|\Psi|}\sum_{\rich{M}\in \{\rich{M}_\psi\ind{2}: \psi\in \Psi\}}\mathbb{E}_{D_n\sim \rich{M}}\left[\left|\widehat{V}_{D_n} - \rich{V}^{\rich{M}}(\rich\rho)\right|\right]\\
        & \ge \frac{\epsilon}{4H}\cdot \left(\frac{1}{|\Psi|}\sum_{\rich{M}\in \{\rich{M}_\psi\ind{1}: \psi\in \Psi\}}\mathbb{P}_{D_n\sim \rich{M}}(\delta\prn{D_n} = 1) + \frac{1}{|\Psi|}\sum_{\rich{M}\in \{\rich{M}_\psi\ind{2}: \psi\in \Psi\}}\mathbb{P}_{D_n\sim \rich{M}}(\delta\prn{D_n} = 0)\right)\\
        & \ge \frac{\epsilon}{4H}\cdot \left(1 - D_{\mathrm{TV}}(\mathbb{P}_n\ind{1}, \mathbb{P}_n\ind{2})\right), 
    \end{align*}
    where in the last inequality we use $\mathbb{P}(E) + \mathbb{Q}(E^c)\ge 1 - D_{\mathrm{TV}}(\mathbb{P}, \mathbb{Q})$ for any event $\cE$. %\ayush{Use the notation \(\cE\) for events. Your current notaton comes very close to expectations}
\end{proof}

Hence we only need to upper bound the TV distance between $\mathbb{P}_n\ind{1}$ and $\mathbb{P}_n\ind{2}$, which is proved in the following lemma.
\ayush{Try to see if you can breka this down into sublemmas}
\CW{If its unnatural to split into lemmas, I think we can also add little section titles within the proof to make it more structured, like \textbf{Part I. XXX}, \textbf{Part II. YYY}, where XXX YYY are the things we're doing in this part.  }

\begin{lemma}
    Suppose for every $\phi\in \Psi$, we have 
    $$|\calX(\phi)|\ge \frac{32|\phi|^4H^3\ophatC{M}{\mu}{\epsilon}{\Phi}^3}{\epsilon^3}.$$
    If $n\le \frac{H}{8\epsilon} \ophatC{M}{\mu}{\epsilon}{\Phi}$, we have
    $$D_{\mathrm{TV}}(\mathbb{P}_n\ind{1}, \mathbb{P}_n\ind{2})\le \frac{1}{2}.$$
\end{lemma}

\begin{proof}
    First of all, we define
    $$\mathbb{P}_n\ind{0}(\{(\sx_i,\sa_i, r_i, \sx_i')\}_{i=1}^n) \triangleq \prod_{i=1}^n \rich{\mu}\ind{0}(\sx_i,\sa_i)\rich{R}\ind{0}(r_i\mid \sx_i,\sa_i)\rich{T}\ind{0}(\sx_i'\mid \sx_i,\sa_i),$$
    where for $\sx\in \calX(\phi)$,
    %\ayush{Why is the following a nicefrak in displayed equation?} 
    \begin{align}
        \rich{\mu}\ind{0}(\sx, \sa) & \triangleq \frac{\mu(\phi, \sa)}{|\calX(\phi)|},\label{eq:sec-lower-bound-mu0}\\
        \rich{T}\ind{0}(\sx'\mid \phi,\sa) & \triangleq \sum_{\sz\in \phi}\mu(\sz\mid \phi, \sa)\rich{T}\ind{1}(\sx'\mid \sz, \sa).\label{eq:sec-lower-bound-T0}
    \end{align}
    and,
    $$\rich{R}\ind{0}(\cdot \mid \sx,\sa) = \begin{cases}
        \delta(1) &\quad \sx = \su_h,\\
        \delta(-1) &\quad \sx = \sv_h,\\
        \frac{1}{2}\delta(1) + \frac{1}{2}\delta(-1) &\quad \text{otherwise}.
    \end{cases}$$
    Then it is easy to see that $\mathbb{P}_n\ind{0}$ is a distribution. Hence we have 
    $$D_{\mathrm{TV}}(\mathbb{P}_n\ind{1}, \mathbb{P}_n\ind{2})\le D_{\mathrm{TV}}(\mathbb{P}_n\ind{1}, \mathbb{P}_n\ind{0}) + D_{\mathrm{TV}}(\mathbb{P}_n\ind{2}, \mathbb{P}_n\ind{0}).$$
    Therefore, if we prove that
    $$\TV(\mathbb{P}_n\ind{1}, \mathbb{P}_n\ind{0})\le \frac{1}{4} \quad\text{and}\quad \TV(\mathbb{P}_n\ind{2}, \mathbb{P}_n\ind{0})\le \frac{1}{4},$$
    then we have the desired property. Without loss of generality, in the following we  only prove
    $$\TV(\mathbb{P}_n\ind{1}, \mathbb{P}_n\ind{0})\le \frac{1}{4}.$$
    We write
    $$\mathbb{P}_n\ind{1}(\{(\sx_i,\sa_i, r_i, \sx_i')\}_{i=1}^n) = \frac{1}{|\Psi|}\sum_{\psi\in\Psi}\prod_{i=1}^n \rich{\mu}_\psi(\sx_i,\sa_i)\rich{R}\ind{1}(r_i \mid \sx_i,\sa_i)\rich{T}_{\psi}\ind{1}(\sx_i'\mid \sx_i,\sa_i),$$
    where $\rich{r}\ind{1}$ is defined in \pref{eq:sec-lower-bound-def-r}. To facilitate the proof, we define
    $$\tilde{\mathbb{P}}_n\ind{1}(\{(\sx_i,\sa_i, r_i, \sx_i')\}_{i=1}^n) = \frac{1}{|\Psi|}\sum_{\psi\in\Psi}\prod_{i=1}^n \rich{\mu}_\psi(\sx_i,\sa_i)\rich{R}\ind{0}(r_i \mid \sx_i,\sa_i)\rich{T}_{\psi}\ind{1}(\sx_i'\mid \sx_i,\sa_i).$$
    When $n\le \nicefrac{H\ophatC{M}{\mu}{\epsilon}{\Phi}}{2\epsilon}$, given the form of $\rich{r}\ind{0}$ and $\rich{r}\ind{1}$, we have
    \begin{align*}
        \TV(\mathbb{P}_n\ind{1}, \tilde{\mathbb{P}}_n\ind{1}) & = \frac{1}{2}\sum_{\{(\sx_i,\sa_i, r_i, \sx_i')\}_{i=1}^n}\left|\mathbb{P}_n\ind{1}(\{(\sx_i,\sa_i, r_i, \sx_i')\}_{i=1}^n - \tilde{\mathbb{P}}_n\ind{1}(\{(\sx_i,\sa_i, r_i, \sx_i')\}_{i=1}^n\right|\\
        &\le \frac{1}{2}\sum_{\{(\sx_i,\sa_i)\}_{i=1}^n}\frac{1}{|\Psi|}\sum_{\psi\in\Psi}\sum_{i=1}^n|\rich{r}\ind{1}(\sx_i,\sa_i) - \rich{r}\ind{0}(\sx_i,\sa_i)|\prod_{i=1}^n \rich{\mu}_\psi(\sx_i,\sa_i)\\
        &\le \frac{1}{2|\Psi|}\sum_{\psi\in\Psi}\sum_{i=1}^n\sum_{(\sx_i,\sa_i)}\rich{\mu}_\psi(\sx_i,\sa_i)|\rich{r}\ind{1}(\sx_i,\sa_i) - \rich{r}\ind{0}(\sx_i,\sa_i)|\\
        &\le \frac{1}{2|\Psi|}\sum_{\psi\in\Psi}\sum_{i=1}^n\sum_{\sx_i}\rich{\mu}_\psi(\sx_i, \ripieval(\sx_i))\frac{\epsilon\indic\{\zeta(\psi(\sx_i))\in\Phiopt)\}}{2H\sum_{\phi\in \Phiopt}\agg{d}^\pieval(\phi)}\\
        & = \frac{n\epsilon}{4H\sum_{\phi\in \Phiopt}\agg{d}^\pieval(\phi)}\sum_{\sz: \zeta(\sz)\in \Phiopt}\mu(\sz, \pieval(\sz))\le \frac{n\epsilon}{4H\ophatC{M}{\mu}{\epsilon}{\Phi}}\sum_{\phi\in \Phiopt} \agg{d}^\pieval(\phi)\le \frac{1}{8}.
    \end{align*}

    Therefore, we obtain
    \begin{equation}\label{eq:sec-lower-bound-tv}\TV(\mathbb{P}_n\ind{1}, \mathbb{P}_n\ind{0})\le \TV(\mathbb{P}_n\ind{1}, \tilde{\mathbb{P}_n\ind{1}}) + \TV(\mathbb{P}_n\ind{0}, \tilde{\mathbb{P}_n\ind{1}})\le \frac{1}{8} + \frac{1}{2}\sqrt{D_{\chi^2}(\tilde{\mathbb{P}}_n\ind{1}\|\mathbb{P}_n\ind{0})}.\end{equation}
    If using \(\mathbb{E}_{0}\) to denote \(\mathbb{E}_{\{(\sx_i,\sa_i, r_i, \sx_i')\}_{i=1}^n\sim \mathbb{P}_n\ind{0}}\), then we have
    \begin{align*}
        &\quad D_{\chi^2}(\tilde{\mathbb{P}}_n\ind{1}\|\mathbb{P}_n\ind{0}) \\ 
        & = \mathbb{E}_{0}\left[\left(\frac{\tilde{\mathbb{P}}_n\ind{1}(\{(\sx_i,\sa_i, r_i, \sx_i')\}_{i=1}^n)}{\mathbb{P}_n\ind{0}(\{(\sx_i,\sa_i, r_i, \sx_i')\}_{i=1}^n)}\right)^2\right] - 1\\
        & = \mathbb{E}_{0}\left[\left(\frac{\frac{1}{|\Psi|}\sum_{\psi\in\Psi}\prod_{i=1}^n \rich{\mu}_{\psi}(\sx_i,\sa_i)\rich{R}\ind{0}(r_i\mid\sx_i,\sa_i)\rich{T}_{\psi}\ind{1}(\sx_i'\mid \sx_i,\sa_i)}{\prod_{i=1}^n \rich{\mu}\ind{0}(\sx_i,\sa_i)\rich{R}\ind{0}(r_i\mid\sx_i,\sa_i)\rich{T}\ind{0}(\sx_i'\mid \sx_i,\sa_i)}\right)^2\right] - 1\\
        & = \mathbb{E}_{0}\left[\left(\frac{\frac{1}{|\Psi|}\sum_{\psi\in\Psi}\prod_{i=1}^n \rich{\mu}_{\psi}(\sx_i,\sa_i)\rich{T}_{\psi}\ind{1}(\sx_i'\mid \sx_i,\sa_i)}{\prod_{i=1}^n \rich{\mu}\ind{0}(\sx_i,\sa_i)\rich{T}\ind{0}(\sx_i'\mid \sx_i,\sa_i)}\right)^2\right] - 1\\
        & = \frac{1}{|\Psi|^2}\sum_{\psi_1, \psi_2\in \Psi}\mathbb{E}_{0}\left[\frac{\prod_{i=1}^n \rich{\mu}_{\psi_1}(\sx_i,\sa_i)\rich{\mu}_{\psi_2}(\sx_i,\sa_i)\rich{T}_{\psi_1}\ind{1}(\sx_i'\mid \sx_i,\sa_i)\rich{T}_{\psi_2}\ind{1}(\sx_i'\mid \sx_i,\sa_i)}{\prod_{i=1}^n\rich{\mu}\ind{0}(\sx_i,\sa_i)^2\rich{T}\ind{0}(\sx_i'\mid \sx_i,\sa_i)^2}\right] - 1\\
        & = \frac{1}{|\Psi|^2}\sum_{\psi_1, \psi_2\in \Psi}\left(\mathbb{E}_{(\sx, \sa)\sim \rich{\mu}\ind{0}, \sx'\in \rich{T}\ind{0}(\cdot\mid \sx, \sa)}\left[\frac{\rich{\mu}_{\psi_1}(\sx,\sa)\rich{\mu}_{\psi_2}(\sx,\sa)\rich{T}_{\psi_1}\ind{1}(\sx'\mid \sx,\sa)\rich{T}_{\psi_2}\ind{1}(\sx'\mid \sx,\sa)}{\rich{\mu}\ind{0}(\sx,\sa)^2\rich{T}\ind{0}(\sx'\mid \sx,\sa)^2}\right]\right)^n - 1
    \end{align*}

According to Jensen's inequality, we obtain
    \begin{align*}
        &\quad \left(\mathbb{E}_{(\sx, \sa)\sim \rich{\mu}\ind{0}, \sx'\in \rich{T}\ind{0}(\cdot\mid \sx, \sa)}\left[\frac{\rich{\mu}_{\psi_1}(\sx,\sa)\rich{\mu}_{\psi_2}(\sx,\sa)\rich{T}_{\psi_1}\ind{1}(\sx'\mid \sx,\sa)\rich{T}_{\psi_2}\ind{1}(\sx'\mid \sx,\sa)}{\rich{\mu}\ind{0}(\sx,\sa)^2\rich{T}\ind{0}(\sx'\mid \sx,\sa)^2}\right]\right)^n\\
        & \le \mathbb{E}_{\phi\sim \mu\ind{0}, \sa\sim \mu\ind{0}(\cdot\mid \phi)}\left(\mathbb{E}_{\sx\sim \rich{\mu}\ind{0}(\cdot\mid \phi, \sa), \sx'\in \rich{T}\ind{0}(\cdot\mid \sx, \sa)}\left[\frac{\rich{\mu}_{\psi_1}(\sx\mid \phi, \sa)\rich{\mu}_{\psi_2}(\sx\mid \phi, \sa)\rich{T}_{\psi_1}\ind{1}(\sx'\mid \sx,\sa)\rich{T}_{\psi_2}\ind{1}(\sx'\mid \sx,\sa)}{\rich{\mu}\ind{0}(\sx\mid \phi, \sa)^2\rich{T}\ind{0}(\sx'\mid \sx,\sa)^2}\right]\right)^n.
    \end{align*}
    We further define
    $$\theta_{\sz_1, \sz_2}\triangleq \frac{|\calX_{\psi_1}(\sz_1)\cap \calX_{\psi_2}(\sz_2)|}{|\calX(\phi)|},\quad \forall \sz_1, \sz_2\in \phi.$$
    According to \pref{eq:sec-lower-bound-mu0}, we know that $\rich{\mu}\ind{0}(\cdot\mid\phi, \sa)$ is a uniform distribution over $\calX(\phi)$, i.e. for any $\sx\in \calX(\phi)$, $\rich{\mu}\ind{0}(\sx\mid\phi, \sa) = \nicefrac{1}{|\calX(\phi)|}$. Additionally, for those $\sx\in \calX_{\psi_1}(\sz_1)\cap \calX_{\psi_2}(\sz_2)$, 
    \begin{align*}
        \rich{\mu}_{\psi_1}(\sx\mid \phi, \sa) & = \mu(\sz_1\mid\phi, \sa)\mu(\sx\mid\sz_1) = \frac{\mu(\sz_1\mid\phi, \sa)}{|\calX_{\psi_1}(\sz_1)|} = \frac{\mu(\sz_1\mid\phi, \sa)|\phi|}{|\calX(\phi)|},\\
        \rich{\mu}_{\psi_2}(\sx\mid \phi, \sa) & = \mu(\sz_2\mid\phi, \sa)\mu(\sx\mid\sz_2) = \frac{\mu(\sz_2\mid\phi, \sa)|\phi|}{|\calX(\phi)|}.
    \end{align*}
    Therefore, we obtain that 
    
    Next, we notice that from \pref{eq:sec-lower-bound-T0}, for any $\sx', \phi, \sa$
    $$\rich{T}\ind{0}(\sx'\mid \phi,\sa) = \sum_{\sz\in \phi}\mu(\sz\mid \phi, \sa)\rich{T}\ind{1}(\sx'\mid \sz, \sa).$$

    Next, we define set 
    \begin{equation}\label{eq:sec-lower-bound-defGamma}\Gamma_{\phi, \sz_1, \sz_2}(\xi)\triangleq \left\{(\psi_1, \psi_2): \theta_{\sz_1, \sz_2}\le \frac{1}{|\phi|^2} + \frac{\xi}{|\phi|}\right\}\end{equation}
    and
    $$\Gamma_\phi(\xi) \triangleq \left\{(\psi_1, \psi_2): \forall \sz_1, \sz_2\in \phi, \theta_{\sz_1, \sz_2}\le \frac{1}{|\phi|^2} + \frac{\xi}{|\phi|}\right\} = \bigcap_{\sz_1, \sz_2\in \phi}\Gamma_{\phi, \sz_1, \sz_2}(\xi),$$
    then we have for any $(\psi_1, \psi_2)\in \Gamma_\phi(\xi)$,
    \begin{align*}
        &\quad \sum_{\sz_1, \sz_2\in \phi}\theta_{\sz_1, \sz_2}\sum_{\sx'}\frac{\mu(\sz_1\mid\phi, \sa)\mu(\sz_2\mid\phi, \sa)|\phi|^2\rich{T}\ind{1}(\sx'\mid \sz_1,\sa)\rich{T}\ind{1}(\sx'\mid \sz_2,\sa)}{\rich{T}\ind{0}(\sx'\mid \phi,\sa)}\\ 
        & \le (1 + |\phi|\xi)\sum_{\sz_1, \sz_2\in \phi}\sum_{\sx'}\frac{\mu(\sz_1\mid\phi, \sa)\mu(\sz_2\mid\phi, \sa)\rich{T}\ind{1}(\sx'\mid \sz_1,\sa)\rich{T}\ind{1}(\sx'\mid \sz_2,\sa)}{\rich{T}\ind{0}(\sx'\mid \phi,\sa)}\\
        & = (1 + |\phi|\xi)\sum_{\sx'}\rich{T}\ind{0}(\sx'\mid \phi,\sa)\sum_{\sz_1, \sz_2\in \phi}\frac{\mu(\sz_1\mid\phi, \sa)\mu(\sz_2\mid\phi, \sa)\rich{T}\ind{1}(\sx'\mid \sz_1,\sa)\rich{T}\ind{1}(\sx'\mid \sz_2,\sa)}{\rich{T}\ind{0}(\sx'\mid \phi,\sa)^2}\\
        & = (1 + |\phi|\xi)\sum_{\sx'}\rich{T}\ind{0}(\sx'\mid \phi,\sa) = 1 + |\phi|\xi.
    \end{align*}
    Additionally, for any $(\psi_1, \psi_2)\in \Psi^2$, noticing that $\theta_{\sz_1, \sz_2}\le 1$ always holds for all $\sz_1, \sz_2$, we have
    \begin{align*}
        &\quad \sum_{\sz_1, \sz_2\in \phi}\theta_{\sz_1, \sz_2}\sum_{\sx'}\frac{\mu(\sz_1\mid\phi, \sa)\mu(\sz_2\mid\phi, \sa)|\phi|^2\rich{T}\ind{1}(\sx'\mid \sz_1,\sa)\rich{T}\ind{1}(\sx'\mid \sz_2,\sa)}{\rich{T}\ind{0}(\sx'\mid \phi,\sa)}\\
        & \le |\phi|^2\sum_{\sz_1, \sz_2\in \phi}\sum_{\sx'}\frac{\mu(\sz_1\mid\phi, \sa)\mu(\sz_2\mid\phi, \sa)\rich{T}\ind{1}(\sx'\mid \sz_1,\sa)\rich{T}\ind{1}(\sx'\mid \sz_2,\sa)}{\rich{T}\ind{0}(\sx'\mid \phi,\sa)}  = |\phi|^2.
    \end{align*}
    Therefore, we obtain that
    \begin{align*}
        &\quad \frac{1}{|\Psi|^2}\sum_{\psi_1, \psi_2\in \Psi}\left(\mathbb{E}_{\sx\sim \rich{\mu}\ind{0}(\cdot\mid \phi, \sa), \sx'\in \rich{T}\ind{0}(\cdot\mid \sx, \sa)}\left[\frac{\rich{\mu}_{\psi_1}(\sx\mid \phi, \sa)\rich{\mu}_{\psi_2}(\sx\mid \phi, \sa)\rich{T}_{\psi_1}\ind{1}(\sx'\mid \sx,\sa)\rich{T}_{\psi_2}\ind{1}(\sx'\mid \sx,\sa)}{\rich{\mu}\ind{0}(\sx\mid \phi, \sa)^2\rich{T}\ind{0}(\sx'\mid \sx,\sa)^2}\right]\right)^n - 1\\
        & \le \frac{1}{|\Psi|^2}\sum_{\psi_1, \psi_2\in \Psi} \left[(1 + |\phi|\xi)^n + \indic\{(\psi_1, \psi_2)\not\in \Gamma_\phi(\xi)\}|\phi|^{2n}\right] - 1.
    \end{align*}
    When $\xi\le \nicefrac{1}{n|\phi|}$, we have $(1 + |\phi|\xi)^n \le 1 + 2|\phi|\xi n$, which indicates that the above formula is 
    $$\le 2|\phi|\xi n + |\phi|^{2n}\frac{1}{|\Psi|^2}\sum_{\psi_1, \psi_2\in \Psi}\indic\{(\psi_1, \psi_2)\not\in \Gamma_\phi(\xi)\}.$$
    Next, according to Lemma \ref{lem:g_phi}, we have
    $$\frac{1}{|\Psi|^2}\sum_{\psi_1, \psi_2\in \Psi} \indic\{\psi_1, \psi_2)\not\in \Gamma_{\phi, \sz_1, \sz_2}(\xi)\} \le \exp(\nicefrac{-2\xi^2 |\calX(\phi)|}{|\phi|}).$$
    Hence,
    $$\frac{1}{|\Psi|^2}\sum_{\psi_1, \psi_2\in \Psi}\indic\{(\psi_1, \psi_2)\not\in \Gamma_\phi(\xi)\}\le |\phi|^2\exp(\nicefrac{-2\xi^2 |\calX(\phi)|}{|\phi|}).$$
    When $|\calX(\phi)|\ge \nicefrac{32|\phi|^4H^3\ophatC{M}{\mu}{\epsilon}{\Phi}^3}{\epsilon^3}$ and $n\le \nicefrac{H\ophatC{M}{\mu}{\epsilon}{\Phi}}{8\epsilon}$, we have
    $$|\calX(\phi)|\ge 16384|\phi|^4n^3\ge 8192|\phi|^4n^2 + 4096(n+1)|\phi|^3n^2\log|\phi|.$$
    Hence if we choose $\xi = \nicefrac{1}{64|\phi|n}$, we obtain
    $$2|\phi|\xi n + |\phi|^{2n}\frac{1}{|\Psi|^2}\sum_{\psi_1, \psi_2\in \Psi}\indic\{(\psi_1, \psi_2)\not\in \Gamma_\phi(\xi)\}\le 2|\phi|\xi n + |\phi|^2\exp(\nicefrac{-2\xi^2 |\calX(\phi)|}{|\phi|})\le \frac{1}{16}.$$
    This indicate that
    $$\frac{1}{|\Psi|^2}\sum_{\psi_1, \psi_2\in \Psi}\left(\mathbb{E}_{\sx\sim \rich{\mu}\ind{0}(\cdot\mid \phi, \sa), \sx'\in \rich{T}\ind{0}(\cdot\mid \sx, \sa)}\left[\frac{\rich{\mu}_{\psi_1}(\sx\mid \phi, \sa)\rich{\mu}_{\psi_2}(\sx\mid \phi, \sa)\rich{T}_{\psi_1}\ind{1}(\sx'\mid \sx,\sa)\rich{T}_{\psi_2}\ind{1}(\sx'\mid \sx,\sa)}{\rich{\mu}\ind{0}(\sx\mid \phi, \sa)^2\rich{T}\ind{0}(\sx'\mid \sx,\sa)^2}\right]\right)^n - 1\le \frac{1}{16},$$
    and hence 
    $$D_{\chi^2}(\tilde{\mathbb{P}}_n\ind{1}\|\mathbb{P}_n\ind{0})\le \frac{1}{16}.$$
    Bringing this inequality back into \pref{eq:sec-lower-bound-tv}, we have
    $$\TV(\mathbb{P}_n\ind{1}~\|~\mathbb{P}_n\ind{0})\le \frac{1}{4}.$$
    This completes the proof of this lemma.
\end{proof}

\begin{lemma}\label{lem:g_phi}
    For $\Gamma_{\phi, \sz_1, \sz_2}(\xi)$ defined in \pref{eq:sec-lower-bound-defGamma}, we have %\ayush{Typically lemma's need more details that just "we have" as this is clearly a placeholder for the fact that you had nothing to say}
    $$\frac{1}{|\Psi|^2}\sum_{\psi_1, \psi_2\in \Psi} \indic\{(\psi_1, \psi_2)\not\in \Gamma_{\phi, \sz_1, \sz_2}(\xi)\} \le \exp(\nicefrac{-2\xi^2|\calX(\phi)|}{|\phi|}).$$
\end{lemma}
\begin{proof}
    We denote $S = |\calX(\phi)|$. Without loss of generality, we assume $\calX(\phi) = [S] = \{1, 2, \cdots, S\}$. Since $\psi_1$ and $\psi_2$ are samples i.i.d.~ according to $\text{Unif}(\Psi)$, without loss of generality we assume $\calX_{\psi_1}(\sz_1) = [\nicefrac{S}{|\phi|}]$. And to prove this lemma, we only need to verify that when $\psi_2\sim \mathrm{Unif}(\Psi)$, we have 
    \begin{equation}\label{eq:sec-lower-bound-high-probability}
        \mathbb{P}\left(|\calX_{\psi_2}(\sz_2)\cap [\nicefrac{S}{|\phi|}]|\in [(\nicefrac{S}{|\phi|^2}+\nicefrac{\xi S}{|\phi|}, \infty)\right)\le \exp(\nicefrac{-2\xi^2S}{|\phi|}).
    \end{equation}
    
    \par Next, we notice that sampling $\psi_2\sim \mathrm{Unif}(\Psi)$ is equivalent of sampling $\calX_{\psi_2}(\sz_2)$ uniformly from all subsets of $[S]$ with exact $\nicefrac{S}{|\phi|}$ elements. Hence we obtain that
    $$\mathbb{P}\left(|\calX_{\psi_2}(\sz_2)\cap [\nicefrac{S}{|\phi|}]|\in [(\nicefrac{S}{|\phi|^2}+\nicefrac{\xi S}{|\phi|}, \infty)\right) = \sum_{t\ge \nicefrac{S}{|\phi|^2} + \nicefrac{\xi S}{|\phi|}}\frac{\binom{\nicefrac{S}{|\phi|}}{t}\binom{S - \nicefrac{S}{|\phi|}}{\nicefrac{S}{|\phi|} - t}}{\binom{S}{\nicefrac{S}{|\phi|}}}.$$
    We further notice that according to Lemma D.7 in \cite{foster2022offline} (also in \cite{hoeffding1994probability}), if we choose $K = N' = \nicefrac{S}{|\phi|}, N = S$, we get %\ayush{Write this lemma statement somewhere for easy reference!}  
\begin{align*}
\sum_{t\ge \nicefrac{S}{|\phi|^2} + \nicefrac{\xi S}{|\phi|}}\frac{\binom{\nicefrac{S}{|\phi|}}{t}\binom{S - \nicefrac{S}{|\phi|}}{\nicefrac{S}{|\phi|} - t}}{\binom{S}{\nicefrac{S}{|\phi|}}}\le \exp(\nicefrac{-2\xi^2S}{|\phi|}).
\end{align*}
    Hence we have $\text{LHS of }\pref{eq:sec-lower-bound-high-probability}\le \exp(\nicefrac{-2\xi^2S}{|\phi|})$. This finishes the proof of this lemma.
\end{proof} 

\begin{lemma}[Lemma D.7 in \cite{foster2022offline}]
    Let $X\sim\mathrm{Hyper}(K, N, N')$ and define $p = K/N$. Then for any $0 < \epsilon < pN'$, we have
    $$\mathbb{P}[X\ge (p + \epsilon)N']\le \exp(-2\epsilon^2N').$$
\end{lemma}

\newpage
\section{Proof of \pref{thm:strongly admissible lower bound}}  
\par In this subsection, we show that admissible data with enough concentrability coefficient is not sufficient for offline RL. To facilitate the proof, we use $d^\pi(\sx, M)$ to denotes the occupancy of state $\sx$ under policy $\pi$ and MDP $M$.

\par We construct the latent MDP $M = (\calZ, \calA, T, H, \rho)$ as follows (this MDP can be viewed in Figure \ref{fig:MDP}): $\calZ = \cup_{h=1}^H\calZ_h$, where $\calZ_{h} = \{\sz_h\inds{1}, \sz_h\inds{2}, \sz_h\inds{3}\}$, and $\calA = \{a_1, a_2\}$. The transition model $T$ is defined as: %\ayush{Fix the exponents in the following? In order to be consistent with the general notation of \(z\inds{1}\), I propose using the notation \(z_{h}\brup{1}, z_{h}\brup{2}, z_{h}\brup{3}\)} 
\begin{align*}
    & T(\cdot\mid \sz_h\inds{1}, \sa_1) = \frac{1}{2}\delta\prn{\sz_{h+1}\inds{1}} + \frac{1}{2}\delta\prn{\sz_{h+1}\inds{2}},\\
    & T(\cdot\mid \sz_h\inds{1}, \sa_2) = \frac{H-2}{2H-2}\delta\prn{\sz_{h+1}\inds{1}} + \frac{H}{2H-2}\delta\prn{\sz_{h+1}\inds{3}},\\
    & T(\cdot \mid \sz_h\inds{2}, \sa_1)  = \delta\prn{\sz_{h+1}\inds{3}},\\
    & T(\cdot\mid \sz_h\inds{2}, \sa_2) = \frac{1}{2}\delta\prn{\sz_{h+1}\inds{1}} + \frac{1}{2H-2}\delta\prn{\sz_{h+1}\inds{2}} + \frac{H-2}{2H-2}\delta\prn{\sz_{h+1}\inds{3}},\\
    &  T(\cdot\mid \sz_h\inds{3}, \sa_2) = T(\cdot\mid \sz_h\inds{3}, \sa_1) = \delta\prn{\sz_{h+1}\inds{3}}.
\end{align*}
The initial distribution $\rho$ is defined as
$$\rho = \frac{H-1}{2H}\delta\prn{\sz_1\inds{1}} + \frac{1}{2H}\delta\prn{\sz_1\inds{2}} + \frac{1}{2}\delta\prn{\sz_1\inds{3}}.$$
%\ascomment{Convert all \(\delta_a\) to \(\delta(a\))} 

We further choose aggregated scheme $\Phi = \cup_{h=1}^H \{\phi_h\inds{1}, \phi_h\inds{2}\}$ with $\phi_h\inds{1} = \{\sz_h\inds{1}, \sz_h\inds{2}\}, \phi_h\inds{2} = \{\sz_h\inds{3}\}$, the policy to be evaluated $\pieval = \delta\prn{\sa_1}$ and the policy used for collecting data $\piexp = \frac{1}{H}\delta\prn{\sa_1} + \frac{H-1}{H}\delta\prn{\sa_2}$. The data collection distribution $\mu$ is chosen to be $d^\piexp$. Then the data collected are admissible data.

For this MDP and data collection distribution, we have the following propositions:
\begin{proposition}
    For MDP $M$, we have
    \begin{enumerate}[label=\((\alph*)\)]
        \item\label{prop:sec-lower-bound-admin-1} The data collection distribution $\mu$ satisfies
        $$\mu(\sz_h\inds{1}, \sa_1) = \frac{H-1}{2^h H^3}, \quad \mu(\sz_h\inds{2}, \sa_1) = \frac{1}{2^h H^3} \quad\text{and}\quad \mu(\sz_h\inds{3}, \sa_1) = \frac{2^h - 1}{2^h H^2}.$$
        \item\label{prop:sec-lower-bound-admin-2} The aggregated concentrability coefficient has lower bound
        $$\ophatC{M}{\phi}{\mu}{\epsilon}\ge \frac{\agg{d}^\pieval(\phi_H\inds{1})}{\sum_{\sz\in \phi_H\inds{1}}\mu(\sz, \pieval(\sz))}\ge \frac{\nicefrac{1}{6}}{\nicefrac{1}{2^HH^2}}\ge 2^{H-3}H^2.$$
    \end{enumerate}
\end{proposition}
\begin{proof}
    We first prove \ref{prop:sec-lower-bound-admin-1}. We can calculate that under policy $\piexp$,
    \begin{align*}
        T(\cdot\mid \sz_h\inds{1}, \piexp(\sz_h\inds{1}))& = \frac{H-1}{2H}\delta\prn{\sz_{h+1}\inds{1}} + \frac{1}{2H}\delta\prn{\sz_{h+1}\inds{2}} + \frac{1}{2}\delta\prn{\sz_{h+1}\inds{3}},\\
        T(\cdot\mid \sz_h\inds{2}, \piexp(\sz_h\inds{2})) & = \frac{H-1}{2H}\delta\prn{\sz_{h+1}\inds{1}} + \frac{1}{2H}\delta\prn{\sz_{h+1}\inds{2}} + \frac{1}{2}\delta\prn{\sz_{h+1}\inds{3}},\\
        T(\cdot\mid \sz_h\inds{3}, \piexp(\sz_h\inds{3})) & = \delta\prn{\sz_{h+1}\inds{3}}.
    \end{align*}
    Hence based on the initial distribution $\rho$, we obtain that 
    \begin{equation}\label{eq:sec-lower-bound-dpiexp}
        d^\piexp(\sz_h\inds{1}) = \frac{H-1}{2^hH^2}, \quad d^\piexp(\sz_h\inds{2}) = \frac{1}{2^h H^2} \quad\text{and}\quad d^\piexp(\sz_h\inds{3}) = \frac{2^h - 1}{2^hH}.
    \end{equation}
    This further implies
    \begin{align*}
        \mu(\sz_h\inds{1}, \sa_1) = \frac{H-1}{2^h H^3}, \quad \mu(\sz_h\inds{2}, \sa_1) = \frac{1}{2^h H^3} \quad\text{and}\quad \mu(\sz_h\inds{3}, \sa_1) = \frac{2^h - 1}{2^h H^2}. 
    \end{align*} 

    Next, we prove \ref{prop:sec-lower-bound-admin-2}. According to \pref{eq:sec-lower-bound-defT} and also our choice of $\mu$,
    \begin{align*}
        &\agg{T}(\phi_{h+1}\inds{1}\mid \phi_h\inds{1}, \sa_1) = \frac{\sum_{\sz_h\in\phi_h\inds{1}, \sz_{h+1}'\in\phi_{h+1}\inds{1}}\mu(\sz_h, \sa_1)T(\sz_{h+1}'\mid \sz_h, \sa_1)}{\sum_{\sz\in\phi_h\inds{1}}\mu(\sz, \sa_1)} \\ 
        &\qquad\ge \frac{\sum_{\sz_{h+1}'\in\phi_{h+1}\inds{1}}\mu(\sz_h\inds{1}, \sa_1)T(\sz_{h+1}'\mid \sz_h\inds{1}, \sa_1)}{\sum_{\sz\in\phi_h\inds{1}}\mu(\sz, \sa_1)}= \frac{\mu(\sz_h\inds{1}, \sa_1)}{\sum_{\sz\in\phi_h\inds{1}}\mu(\sz, \sa_1)} = \frac{H-1}{H-1 + 1} = \frac{H-1}{H}.
    \end{align*}
    This implies that the aggregated state's occupancy $\agg{d}^\pieval(\phi_H\inds{1})$ satisfies
    \begin{align*}
        \agg{d}^\pieval(\phi_H\inds{1})\ge \agg{d}^\pieval(\phi_1\inds{1})\prod_{h=1}^{H-1}\agg{T}(\phi_{h+1}\inds{1}\mid \phi_h\inds{1}, \sa_1)\ge \frac{1}{2}\left(\frac{H-1}{H}\right)^{H-1}\ge \frac{1}{2e}\ge \frac{1}{6}.
    \end{align*}
    Hence when $\epsilon\le \nicefrac{1}{6}$, we have
    \begin{align*}
        \ophatC{M}{\phi}{\mu}{\epsilon}\ge \frac{\agg{d}^\pieval(\phi_H\inds{1})}{\sum_{\sz\in \phi_H\inds{1}}\mu(\sz, \pieval(\sz))}\ge \frac{\nicefrac{1}{6}}{\nicefrac{1}{2^HH^2}}\ge 2^{H-3}H^2.
    \end{align*}
\end{proof}

\begin{theorem}\label{thm:sec-lower-bound-admissible}
    When $H\ge 4$. There exists a class of MDPs where the concentrability coefficient of each instance is bounded by $32H$. For any algorithm taking $\nicefrac{2^{H-6}H^3}{\epsilon}$ number of offline samples, there must exist $\rich{M}$ in this class such that if the samples are according to $d^\ripiexp(\cdot; \rich{M})$, the algorithm will induce estimation error $\nicefrac{\epsilon}{(8H)}$ in $\rich{M}$.
\end{theorem}

\begin{proof}
    We consider the class constructed for proof of \pref{thm:instance_lower_bound} : $\{\rich{M}_\psi\ind{1}: \psi\in\Psi\}\cup\{\rich{M}_\psi\ind{2}: \psi\in\Psi\}$. Under our current construction, the sampling distribution over rich observations is $\rich{\mu}_\psi(\sx, \sa) = \nicefrac{\mu(\psi(\sz), \sa)}{|\calX_\psi(\sz)|}$. And \pref{thm:instance_lower_bound} indicates that for $\epsilon\le \nicefrac{1}{6}$, for any algorithm using less than
    $$\frac{H\ophatC{M}{\phi}{\mu}{\epsilon}}{8\epsilon}\ge 2^{H-6}\frac{H^3}{\epsilon}$$
    samples, there must exist some $\psi\in\Phi$ such that if the samples are according to $\rich{\mu}_\psi$, the algorithm will have error greater than $\nicefrac{\epsilon}{8H}$ in  $\rich{M}_\psi\ind{1}$ or $\rich{M}_\psi\ind{2}$.

    \par Our next observation is that according to \ref{lem:sec-lower-bound-latent-MDP-d} of \pref{prop:sec-lower-bound-latent-MDP},
    we have $d^\piexp(\sz; M\ind{1})\le d^\piexp(\sz; M)$ for any $\sz\in\calZ$. Hence we obtain that for any $\sx\in\calX\backslash \{\su, \sv, \sw\}_{h=1}^H$,
    $$d^{\ripiexp}(\sx; \rich{M}_\psi\ind{1}) = \frac{d^\piexp(\psi(\sx); M)}{|\calX_\psi(\sz)|}\le \frac{d^\piexp(\psi(\sx); M)}{|\calX_\psi(\sz)|}.$$
    This also implies
    $$d^{\ripiexp}(\sx, \sa; \rich{M}_\psi\ind{1}) = d^{\ripiexp}(\sx; \rich{M}_\psi\ind{1})\piexp(\sa\mid\sx)\le \frac{d^\piexp(\psi(\sx); M)\piexp(\sa\mid\sx)}{|\calX_\psi(\sz)|} = \frac{d^\piexp(\psi(\sx), \sa; M)}{|\calX_\psi(\sz)|} = \rich{\mu}_\psi(\sx, \sa).$$
    Similarly, we can also obtain that
    $$d^{\ripiexp}(\sx, \sa; \rich{M}_\psi\ind{2})\le \rich{\mu}_\psi(\sx, \sa).$$
    Hence for any algorithm using less than $\nicefrac{2^{H-6}H^3}{\epsilon}$ number of samples, there must exists some $\rich{M}\in \{\rich{M}_\psi\ind{1}: \psi\in\Psi\}\cup\{\rich{M}_\psi\ind{2}: \psi\in\Psi\}$ such that if the samples are according to $d^{\ripiexp}(\cdot \mid \rich{M})$, the estimation error is at least $\nicefrac{\epsilon}{(8H)}$

    \par Finally, Lemma \ref{lem:sec-lower-bound-coverage} indicates that for any $\rich{M}\in \{\rich{M}_\psi\ind{1}: \psi\in\Psi\}\cup\{\rich{M}_\psi\ind{2}: \psi\in\Psi\}$, the concentrability coefficient is upper bounded by $32H$.
\end{proof}

\begin{lemma}\label{lem:sec-lower-bound-coverage}
    For any $\rich{M}\in \{\rich{M}_\psi\ind{1}:\psi\in\Psi\}\cup\{\rich{M}_\psi\ind{2}:\psi\in\Psi\}$, the concentrability coefficients of $\rich{M}$ of policy $\ripieval$ under distribution $\rich{d}^\ripieval(\cdot; \rich{M})$ are upper bounded by $32H$. %\ayush{This lemma is vague is concentrability coefficient is defined for a policy \(\pieval\) w.r.t. an offline policy}  
\end{lemma}

\begin{proof} 
Without loss of generality, we only prove for $\rich{M}_\psi\ind{1}$ (the proof for $\rich{M}_\psi\ind{2}$ is similar). Suppose $\ripieval$ and $\ripiexp$ are policies over $\rich{M}_\psi\ind{1}$ such that $\ripieval(\sx) = \pieval(\psi(\sx))$ and $\ripiexp(\sx) = \piexp(\psi(\sx))$. In the following, we use $\rich{d}^\pi(\cdot; \rich{M}_\psi\ind{1}), d^\pi(\cdot; M\ind{1})$ and $d^\pi(\cdot; M)$ to denote the occupancy of policy $\pi$ under MDP $\rich{M}_\psi\ind{1}, M\ind{1}$ and $M$. According to \ref{lem:sec-lower-bound-Q-3} in \pref{prop:sec-lower-bound-Q}, we have 
\begin{align*} 
    \frac{\rich{d}^{\ripieval}(\sx; \rich{M}_\psi\ind{1})}{\rich{d}^{\ripiexp}(\sx; \rich{M}_\psi\ind{2})} = \frac{\nicefrac{d^\pieval(\sz; M\ind{1})}{|\calX_\psi(\sz)|}}{\nicefrac{d^\piexp(\sz; M\ind{1})}{|\calX_\psi(\sz)|}} = \frac{d^\pieval(\sz; M\ind{1})}{d^\piexp(\sz; M\ind{1})}.
\end{align*}
Therefore, to show an upper bound for $\rich{M}_\psi\ind{1}$, we only need to prove
\begin{enumerate}[label=\((\alph*)\)]
    \item \label{item:sec-lower-bound-da} For any $\sz\in\calZ$, we have $16H\cdot d^\piexp(\sz; M\ind{1})\ge d^\pieval(\sz; M\ind{1})$; 
    \item \label{item:sec-lower-bound-db} For any $\sz\in \{\su_h, \sv_h, \sw_h\}_{h=1}^H$, we have $32H\cdot d^\piexp(\sz; M\ind{1})\ge d^\pieval(\sz; M\ind{1})$.
\end{enumerate}

First we verify \ref{item:sec-lower-bound-da}. According to \ref{lem:sec-lower-bound-latent-MDP-d} in \pref{prop:sec-lower-bound-latent-MDP}, we have 
$$\frac{d^\pieval(\sz; M\ind{1})}{d^\piexp(\sz; M\ind{1})}\le 16\cdot \frac{d^\pieval(\sz; M)}{d^\piexp(\sz; M)}.$$
Hence we only need to verify $d^\pieval(\sz; M)\le H\cdot d^\piexp(\sz; M)$ for any $\sz\in\calZ$. Our construction implies
$$d^\pieval(\sz_1\inds{1}; M) = \frac{H-1}{2H^2},\quad d^\pieval_M(\sz_1\inds{2}) = \frac{1}{2H^2},\quad d_{M}^\pieval(\sz_h\inds{3})\le 1$$
and  
$$d^\pieval(\sz_h\inds{1}; M) = \frac{H-1}{2^hH^2}, \quad d^\pieval_M(\sz_h\inds{2}) = \frac{H-1}{2^hH^2}, \quad d_{M}^\pieval(\sz_h\inds{3})\le 1\quad \forall 2\le h\le H.$$
Compared with \pref{eq:sec-lower-bound-dpiexp}, we obtain that $d^\pieval(\sz; M)\le H\cdot d^\piexp(\sz; M)$.

Next, we verify \ref{item:sec-lower-bound-db}. We first observe that according to transitions of $M\ind{1}$, we have
\begin{align*}
    d^\pieval(\sw_h; M\ind{1}) = d^\pieval(\su_{h-1}; M\ind{1}) + d^\pieval(\sv_{h-1}; M\ind{1}) + d^\pieval(\sw_{h-1}; M\ind{1}),\\
    d^\piexp(\sw_h; M\ind{1}) = d^\piexp(\su_{h-1}; M\ind{1}) + d^\piexp(\sv_{h-1}; M\ind{1}) + d^\piexp(\sw_{h-1}; M\ind{1}).
\end{align*}
Therefore, we only need to verify for $\sz = \su_h$ and $\sz = \sv_h$. Without loss of generality we only prove for $\sz = \su_h$. We write
\begin{align*}
    d^\piexp(\su_h; M\ind{1}) & = \sum_{\sz\in \calZ_{h-1}} d^\piexp(\sz; M\ind{1})T\ind{1}(\su_h\mid \sz, \piexp(\su_h)),\\
    d^\pieval(\su_h; M\ind{1}) & = \sum_{\sz\in \calZ_{h-1}} d^\pieval(\sz; M\ind{1})T\ind{1}(\su_h\mid \sz, \pieval(\su_h)).
\end{align*}
Additionally, \pref{eq:sec-lower-bound-bound} and \pref{eq:sec-lower-bound-transition} gives that for any $\sz\in\calZ_{H-1}, \sa\in\calA$,
$$\frac{3}{4H}\le T\ind{1}(\su_h\mid \sz, \sa)\le \frac{5}{4H},$$
which implies 
$$T\ind{1}(\su_h\mid \sz, \pieval(\su_h))\le 2\cdot T\ind{1}(\su_h\mid \sz, \piexp(\su_h)).$$
Therefore, noticing from \ref{item:sec-lower-bound-da}, we have 
$$d^\piexp(\sz; M\ind{1})\ge 16\cdot d^\pieval(\sz; M\ind{1}), \quad \forall \sa\in\calZ_{h-1}.$$
Bringing these together, we obtain that \ref{item:sec-lower-bound-db} for $\sz = \su_h$.
\end{proof}

\begin{figure}
    \caption{Hard Case for Admissible Data}
    \label{fig:MDP}
    \centering
    \includegraphics[width = \textwidth]{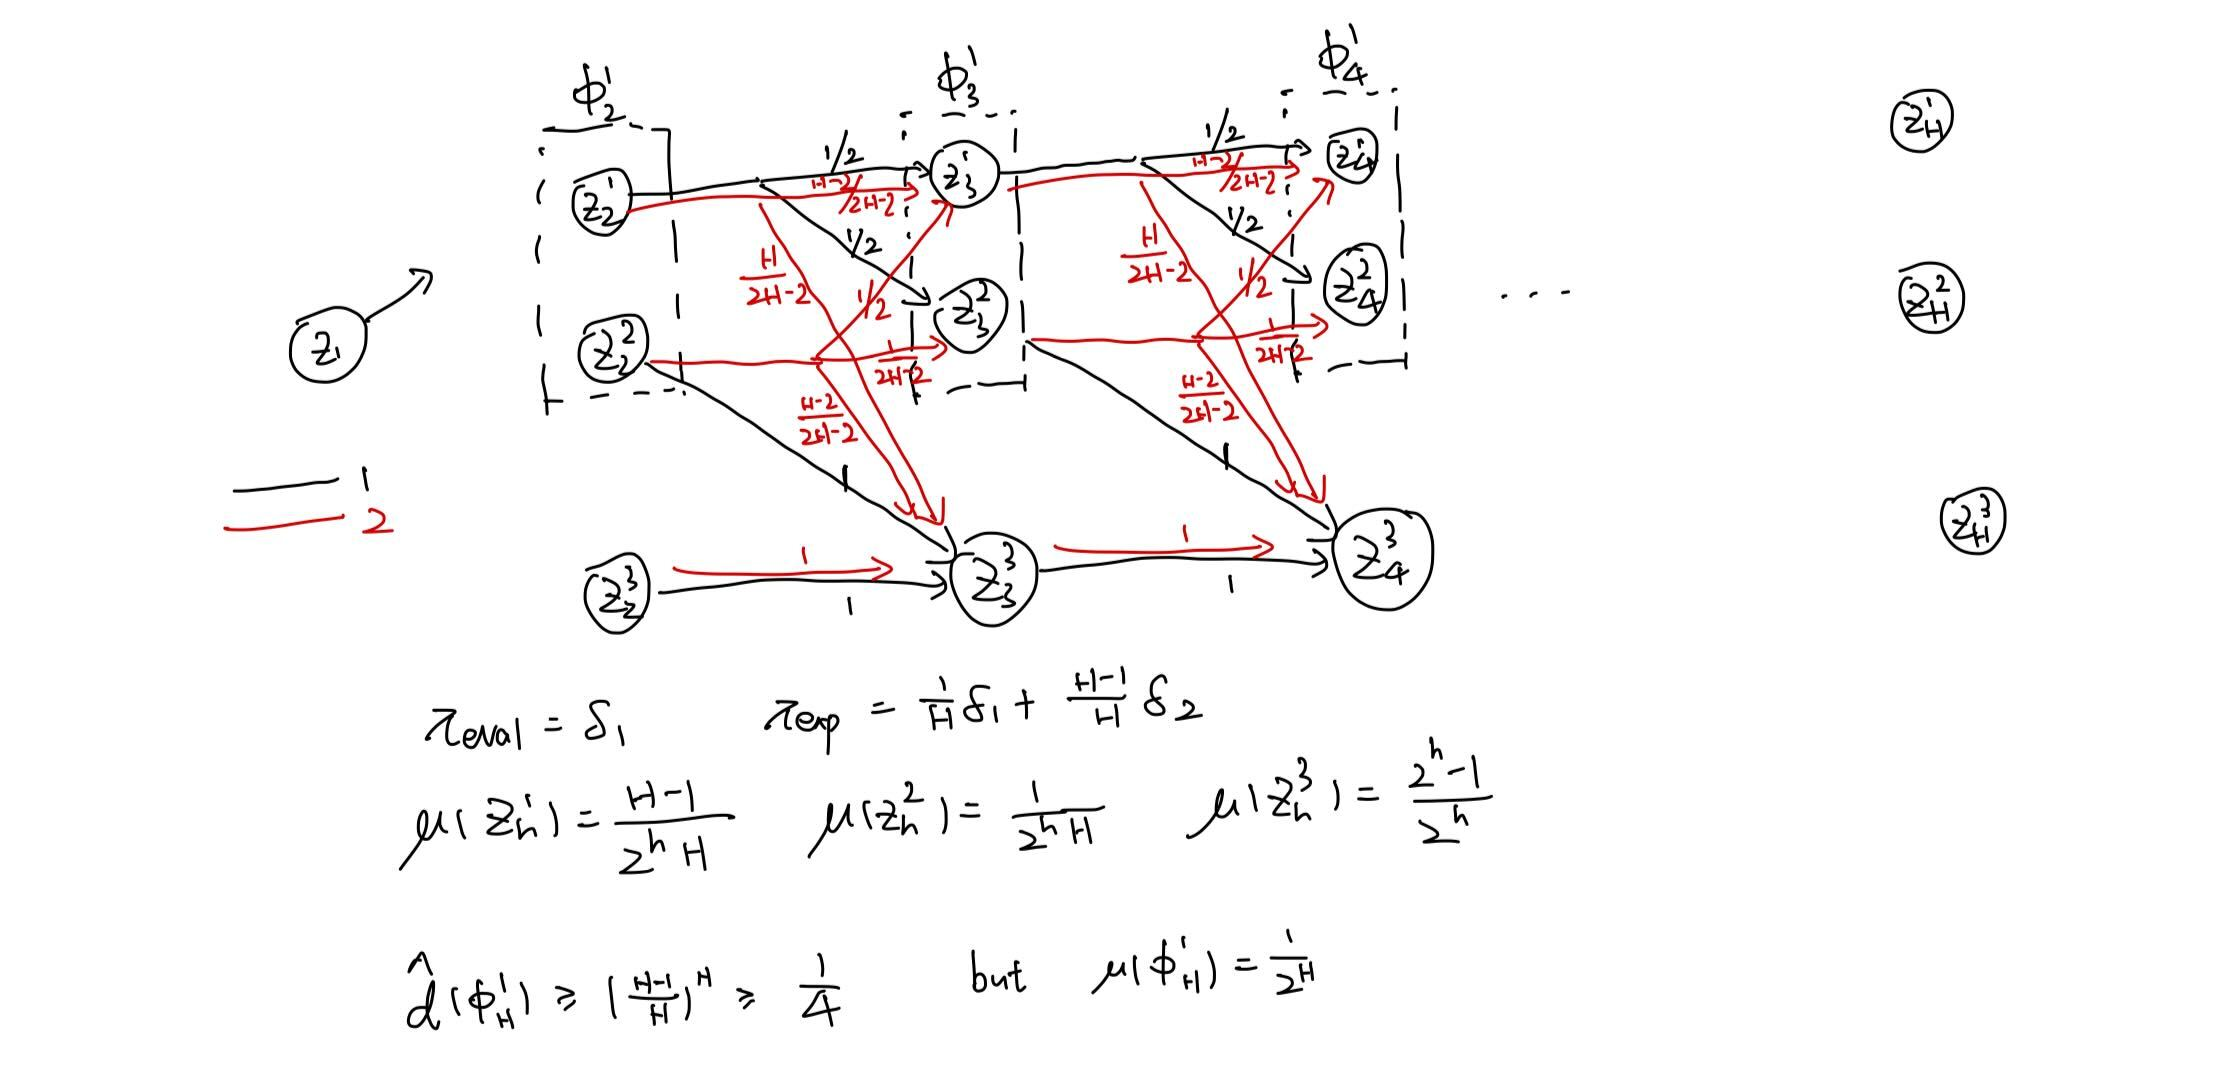}
\end{figure}

\clearpage
